# Supplementary material for: CSCO: Connectivity Search of Convolutional Operators
Source: arXiv:2404.17152 source file (2025-03-25)
Supplement: Supplementary file 1 [file 10_Supplementary.tex]

\section{Supplementary Material}
This supplementary material attaches the detailed configurations and core implementation of DSWiring on CIFAR-10 to provide a better understanding of our proposed method. 
The implementation contains both search code and evaluation code for better demonstration of our method.
Full code for reproducing ImageNet results will be open-sourced upon acceptance of the paper.

\subsection{Search Settings}
We illustrate the detailed search settings as follows:

\noindent \textbf{CIFAR-10.} For CIFAR-10, we employ a ResNet-20 style setting~\cite{he2016deep} where we stack 3 cells in each stage to construct the final CNN architecture. In each stage, we adopt 16, 32, 64 filters, respectively. We train each candidate architecture on 50\% of the CIFAR-10 dataset for 15 epochs with initial learning rate 0.1 and batch size 128 via cosine learning rate schedule~\cite{loshchilov2017sgdr}.

\noindent \textbf{ImageNet.} For ImageNet, we follow the positional settings of DARTS~\cite{liu2018darts} yet shrink the channel by applying 0.5$\times$ width multiplier. In each stage, we adopt 16, 32, 64, 128 filters, respectively during search. We randomly select 50 out of 1000 classes from ImageNet-1K as the proxy dataset following the intuition of FBNet~\cite{wu2019fbnet} and train each candidate architecture for 10 epochs with learning rate 0.1 and batch size 128 via cosine learning rate schedule. 
Note that exponential moving average (EMA) is employed to increase the stability of architecture evaluation.

\subsection{Details of Metropolis-Hastings Evolutionary Search}
We first demonstrate the details of Metropolis-Hastings Evolutionary Search (MH-ES) algorithm in Algorithm \ref{algo:mh_es}.

\begin{algorithm}
    \caption{Metropolis-Hastings Evolutionary Search}
    \label{alg:mh_ea}
    \begin{algorithmic}[1]
        \REQUIRE{Number of Evolution Rounds $\mathbf{R}$; Population Size $P$;
        Number of Stages $K$; Initial Population Size $P_0$;
        Initial temperature $T_0$}
        %\STATE \textbf{begin}
        \STATE Sample $P_0$ candidate architectures, select the best one (i.e., with the highest predictive performance) as parent architectures $\mathbf{G}_{0}$. Set $Score$ to be the predictive performance of $\mathbf{G}_{0}$
        \FOR {$r = 1$ to $R$}
        \STATE Set temperature $T^r=T_0 \cdot \frac{1+\cos{(r\pi / R)}}{2}$
        \STATE Obtain a population of $P$ child architectures via mutation in the mutation space. 
        \STATE Select the one with best predictive performance $Score'$ as $\mathbf{G}$.
        \IF{$Score'>Score$ }
            \STATE $Score=Score'$, $\mathbf{G}_{r+1} = \mathbf{G}$
        \ELSE
            \STATE Generate MH acceptance-rejection ratio: $AC$ $\sim$ $B\Big(1, \exp\big((Score' - Score)/T^r\big)\Big)$
            \IF{AC == 1}
            \STATE Update current best score and parent architecture:
            $Score=Score'$, $\mathbf{G}_{r+1} = \mathbf{G}$
            \ELSE 
            \STATE Preserve the current best parent architecture. $\mathbf{G}_{r+1}=\mathbf{G}_{r}$
            \ENDIF
        \ENDIF
        \ENDFOR
    \end{algorithmic}
    \label{algo:mh_es}
\end{algorithm}
Notably, the initial temperature $T_0$ is an important hyperparameter to tune. For example, setting $T_0 \to 0$ yields local search, as it rejects all child architectures in the mutation space and only focus on exploring the locality in the structural wiring space. When $T_0 \to \infty$, MH-ES never accepts weaker solution and generalizes to Evolutionary Search.

Next, we approach the design intuitions of MH-ES.
The design of MH-ES algorithm is largely intuited by Markov Chain Monte Carlo (MCMC).
MCMC is a crucial technique to obtain promising cells in a solution space.
Here, we extend the analysis of this algorithm by covering more details on the definition of Markov Chains, deriving the expression of Metropolis-Hastings acceptance-rejection ratio that inspires our proposed MH-ES.

\noindent \textbf{Formulation of Markov Chain.}
The exploration problem on a structural wiring design space can be defined as an optimization on a Markov Chain over state space $\mathbf{S}: (\mathcal{G}^{(1)}, \mathcal{G}^{(2)}, ..., \mathcal{G}^{(K)})\subset G^{K\times |G|}$ and transition probability matrix $\mathbf{P}: P_{i,j} \propto \exp\Big(\big(Perf(\mathbf{S}_{j})-Perf(\mathbf{S}_{i})\big)/T\Big)$. 
In DSWiring, the state space is the structural wiring design space, and the transition probability denotes the probability of transiting from one candidate architecture to another.
We first verify the properties below:
\begin{itemize}
    \item The defined Markov Chain is finite. This is obvious as the number of candidate architectures in the structural wiring design space is finite.
    \item The defined Markov Chain is irreducible. Since we assign a non-zero transition probability from one state to another. Thus, the defined Markov chain cannot be reduced to some simpler Markov Chains by removing states.
    \item The defined Markov Chain is aperiodic. We observe that the transition probability matrix $\textbf{P}$ enables the Markov Chain to move toward the states which have a higher score (i.e., predicted performance).
    Thus, it is impossible that the Markov Chain can periodically traverse to the same state and get stuck in an infinite loop during MCMC optimization.
\end{itemize}
Thus, following \textit{the fundamental theorem of Markov Chains}, any irreducible, finite, and aperiodic Markov Chain has a unique stationary distribution.

From the fact that $\mathbf{\pi} = \mathbf{\pi} \mathbf{P}$, it is easy to derive the following system of equations:
\begin{equation}
    \pi_{j} = [\pi \mathbf{P}]_{j} = \sum_{ij}{\pi_{i}P_{ij}} .
\end{equation}
This system admits the solution:
\begin{equation}
\label{eq:soln_pi}
\pi_{i}=\exp\Big(\big(Perf(\mathbf{S}_{i})\big)/T\Big) / Z.   
\end{equation}
where $Z=\sum_{i}\pi_{i}$ is a normalization term.
Following the property of defined Markov Chains, we can see that the above solution is a unique stationary distribution.

\paragraph{Metropolis Algorithm.}
Following the original Metropolis algorithm~\cite{metropolis1953equation}, we use $p$ to denote the target stationary distribution, and use $q$ to denote the proposal distribution.
As is common in the MCMC literature, $q$ is often defined as a symmetric proposal which satisfies the following condition:
\begin{equation}
    \label{eq:symm}
    q(x^{(i)}|x^*) = q(x^{*}|x^{(i)}) ,
\end{equation}
where $x^{*}, x^{(i)}$ are two arbitrary examples in the defined state space. Typically, $x^{*}$ is used to denote the candidate samples to be drawn from the proposal distribution, given priors $x^{(i)}$.
Following the definition of acceptance-rejection ratio definition in the original Metropolis Algorithm, we have
\begin{equation}
    A(x^{(i)}, x^{*}) = \min(1, \frac{p(x^{*})q(x^{(i)}|x^*)}{p(x^{(i)})q(x^{*}|x^{(i)})}) = \min(1, \frac{p(x^*)}{p(x^{(i)})}) .
\end{equation}
The last equality is derived through the symmetric proposal definition defined in Eq.~\ref{eq:symm}.
By plugging in the stationary distribution derived in Eq.~\ref{eq:soln_pi}, the acceptance-rejection ratio for the MCMC optimization can be expressed as
\begin{equation}
    \label{eq:ac_ratio}
    A(x^{(i)}, x^{*}) = \min(1, \exp\Big(\big(Perf(x^{*})-Perf(x^{(i)}\big)/T\Big)) .
\end{equation}
The acceptance-rejection ratio defined in Eq.~\ref{eq:ac_ratio} corresponds to line 9 in Algorithm 1. This acceptance-rejection method can be plugged into Evolutionary Search thus inspires our proposed MH-ES.

\subsection{Resource Consumption}
The resource consumption includes search cost (i.e., the process of sampling models to train the predictor), model selection cost (i.e., the process of selecting the best model) and evaluation cost. 
All the architecture search are performed on NVIDIA RTX A5000 with 24GB memory.
We elaborate on the resource consumption as follows:

\noindent \textbf{Search Cost.} We maintain a fixed search cost of 4 GPU days for both CIFAR-10 and ImageNet. This yields a total of $\sim$ 800 candidate architectures sampled to train the performance predictor.

\noindent \textbf{Model Selection Cost.}
For CIFAR-10, we evaluate the top-5 models for 100 epochs each to select the best model. This takes $\sim$ 0.33 GPU days to complete.
For ImageNet, we evaluate the top-5 models on ImageNet-1K for 10 epochs each to select the best model. This takes $\sim$ 1 GPU day to complete.

\noindent \textbf{Evaluation Cost.} 
For training CIFAR-10 architectures, we train on NVIDIA RTX A5000 GPU and it takes around $\sim0.75$ GPU day to complete a 600-epoch training pipeline following DARTS~\cite{liu2018darts}.
For training ImageNet architectures, we use 2 NVIDIA RTX A5000 GPUs and it takes $\sim5$ GPU days to complete a 300-epoch training pipeline following DARTS~\cite{liu2018darts}.

\noindent \textbf{Hyperparameter Tuning Cost.} We carry light hyperparameter tuning and re-run the overall experimental process for 3$\sim$4 times to achieve the best result. This takes an overall $15\sim20$ GPU days to fully develop.
